# Supplementary material for: Statistical mechanics guides the motions of cm scale objects
Source: arXiv:1805.10812 source file (2018-05-28)
Supplement: Supplementary file 1 [file Boltzmann_atWork_SI.pdf]

# Supplemental material for statistical mechanics guides the motions of cm scale objects

S. Siriroj,[1] P. Simakachorn,[1,2] N. Khumtong,[2] T. Sukhonthamethirat,[2] S. Chaiyachad,[1,3] P. Chanprakhon,[1,3] K. Chanthorn,[1,3] S. Dawprateep,[1,3] T. Eknapakul,[1,3] I. Fongkaew,[1,3] C. Jaisuk,[1,3] T. Jampreecha,[1,3] W. Jindata,[1,3] Y. Kaeokhamchan,[1,3] T. Kongnok,[1,3] P. Laohana,[1,3] K. Lapawer,[1,3] S. Lowpa,[1,3] A. Mooltang,[1,3] S. Musikajaroen,[1,3] S. Nathabumroong,[1,3] A. Panpar,[1,3] S. Phumying,[1,3] S. Polin,[1,3] A. Rasritat,[1,3] A. Ritwiset,[1,3] W. Saengsui,[1,3] W. Saenrang,[1,3] T. Saisopa,[1,3] S. Sangphet,[1,3] T. Sawasdee,[1,3] S. Sonsupap,[1,3] S. Suksombat,[1,3] T. Suyuporn,[1,3] M. Tepakidareekul,[1,3] T. Thiwatwaranikul,[1,3] P. Tipsawat,[1,3] S. Waiprasoet,[1,3] and W. Meevasana[1,3,*]

[1]*School of Physics, Suranaree University of Technology, Nakhon Ratchasima, 30000, Thailand*
[2]*SCiUS program, Suranaree University of Technology and Rajsima Wittayalai School, Nakhon Ratchasima, 30000, Thailand*
[3]*Thailand Center of Excellence in Physics, CHE, Bangkok 10400, Thailand*

(Dated: May 11, 2018)

## I. PROBABILITY AS A FUNCTION OF DROPPING HEIGHT FOR A REGULAR DIE

From the introduction, we wrote "Tossing a die from a decent height on a hard floor is generally thought as a random process." In this section, we would like to experimentally investigate on the height which makes the outcome random enough while having the initial condition to be (almost) the same. We should emphasize here that in principle of classical mechanics, the outcome should be the same with the exact same initial condition; however, since phase space can be very complex (e.g. barbell study [2]), a slight difference in initial condition can give a big difference in the motion. For our setup here, we dropped a cubic die (Vegas grade) with face 1 up from various heights and measured the probability of getting face 1 up again in the final configuration. As shown in Fig. S1, when the height is zero, the probability outcome in getting face 1 up is trivially 1. Then, the probability becomes smaller upon increasing the dropping height. When the dropping height becomes larger than the die length, the probability then becomes close to 1/6 (solid line in Fig. S1); this is the region where we assume the randomness. For our measurements as shown in Fig. 2, to ensure the randomness of their motions, we then chose to drop the dice from the height around 27 cm which is well larger than all the die lengths.

## II. SHORT REVIEW ABOUT THE DERIVATION OF BOLTZMANN DISTRIBUTION

The Boltzmann distribution of a system at equilibrium with a total number of particles $N = \sum_i n_i$ and total energy $E = \sum_i \varepsilon_i n_i$ (for all energy states $\varepsilon_i$) can be derived by maximizing the entropy $S = k \ln W$ [1].

The number of microstates W is given by

$$W = \frac{N!}{n_1!n_2!n_3!\cdots} \tag{1}$$

Here, we can maximize the entropy by maximizing $\ln W$. By using the Stirling's approximation,

$$\ln W \cong N \ln N - \sum_i n_i \ln n_i - \left( N - \sum_i n_i \right) \tag{2}$$

Since $N = \sum_i n_i$, then

$$\ln W \cong N \ln N - \sum_i n_i \ln n_i \tag{3}$$

After taking the derivative where N is a constant,

$$d(\ln W) = -\sum_i (1 + \ln n_i) dn_i = -\sum_i (\ln n_i) dn_i \tag{4}$$

*Authors to whom correspondence should be addressed. Electronic addresses: worawat@g.sut.ac.th

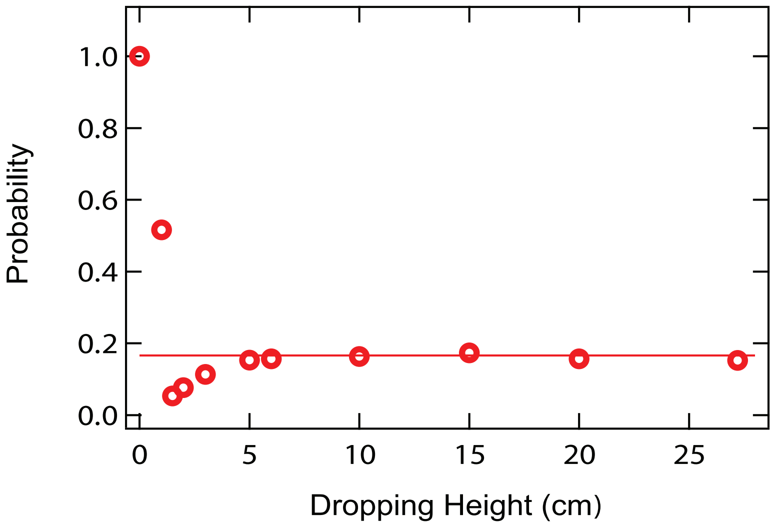


FIG. 1: Probability of a die ending up with the same face up as a function of the dropping height. Solid line shows probability of 1/6, representing the region with random outcome.

Since we are maximizing the entropy under the constraints that $N = \sum_i n_i = const$ and $E = \sum_i \varepsilon_i n_i = const$, we then use Lagrange multipliers $\alpha$ and $\beta$ in this maximization by adding the constraints $dN = \sum_i dn_i = 0$ and $dE = \sum_i \varepsilon_i dn_i = 0$ to the equation. And we can maximize $\ln W$ by setting $d \ln W = 0$.

$$d(\ln W) = -\sum_i (\ln n_i) dn_i - \alpha \sum_i dn_i - \beta \sum_i \varepsilon_i dn_i = 0 \tag{5}$$

$$-\sum_i (\ln n_i + \alpha + \beta \varepsilon_i)\, dn_i = 0 \tag{6}$$

To satisfy this condition in any cases, $\ln n_i + \alpha + \beta\varepsilon_i = 0$ and

$$n_i = e^{-\alpha} e^{-\beta \varepsilon_i}. \tag{7}$$

With $N = \sum_i n_i$ and definition of temperature T, we then arrive with

$$n_i = \frac{N}{Z} e^{-\varepsilon_i/kT} \tag{8}$$

where the partition $Z = \sum_i e^{-\varepsilon_i/kT}$.

## III. DERIVATION OF AVERAGE ENERGY, EQ. (6)

From eq. (5), the total energy of a die is given by $\varepsilon_d = \varepsilon(\omega_i, p_i, r, \theta, \phi) = \sum_{i=1}^{3} \frac{p_i^2}{2m} + \sum_{j=1}^{3} \frac{1}{2} I_j \omega_j^2 + mgr\cos\theta$.

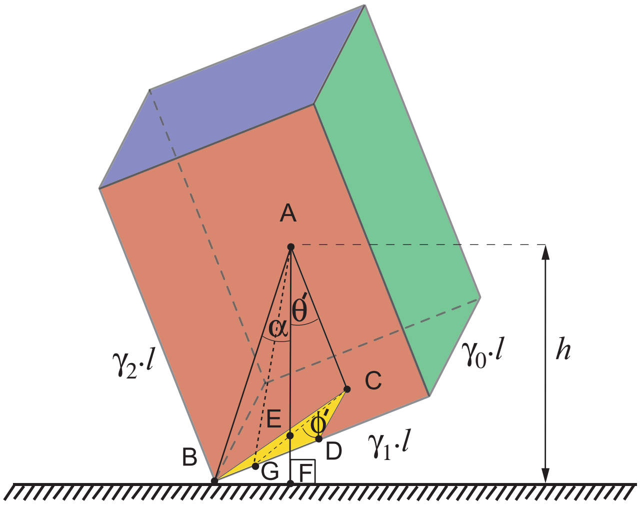


FIG. 2: Diagram in Fig. 3(c) with more variables, points and angles for calculation.

Hence the average energy $\langle \varepsilon_d \rangle$ can be calculated from:

$$
\begin{aligned}
\langle \varepsilon_d \rangle &= \frac{\int\int\int \varepsilon(\omega_i p_i, r, \theta, \phi) \cdot e^{-\varepsilon(\omega_i p_i, r, \theta, \phi)/\kappa\tau} d^3p d^3\omega d^3r}{\int\int\int e^{-\varepsilon(\omega_i p_i, r, \theta, \phi)/\kappa\tau} d^3p d^3\omega d^3r} \\
&= \frac{\int\int\int (\sum_{i=1}^{3} \frac{p_i^2}{2m} + \sum_{j=1}^{3} \frac{1}{2} I_j \omega_j^2 + mgr\cos\theta) \cdot e^{-\varepsilon(\omega_i p_i, r, \theta, \phi)/\kappa\tau} d^3p d^3\omega d^3r}{\int\int\int e^{-\varepsilon(\omega_i p_i, r, \theta, \phi)/\kappa\tau} d^3p d^3\omega d^3r} \\
&= \sum_{i=1}^{3} \left( \frac{\int_0^\infty \frac{p_i^2}{2m} e^{-\frac{p_i^2}{2m}/\kappa\tau} dp_i}{\int_0^\infty e^{-\frac{p_i^2}{2m}/\kappa\tau} dp_i} \right) + \sum_{j=1}^{3} \left( \frac{\int_0^\infty \frac{1}{2} I_j \omega_j^2 e^{-\frac{1}{2} I_j \omega_j^2/\kappa\tau} d\omega_j}{\int_0^\infty e^{\frac{1}{2} I_j \omega_j^2/\kappa\tau} d\omega_j} \right) + \frac{\int_{r=0}^{\infty} \int_{\theta=0}^{\pi/2} \int_{\phi=0}^{2\pi} mgr\cos(\theta) \cdot e^{-mgr\cos(\theta)/\kappa\tau} d^3r}{\int\int\int e^{-mgr\cos(\theta)/\kappa\tau} d^3r} \\
&= 3\left(\frac{\kappa\tau}{2}\right) + 3\left(\frac{\kappa\tau}{2}\right) + \frac{\int_{r=0}^{\infty} \int_{\theta=0}^{\pi/2} \int_{\phi=0}^{2\pi} mgr\cos(\theta) \cdot e^{-mgr\cos(\theta)/\kappa\tau} d^3r}{\int\int\int e^{-mgr\cos(\theta)/\kappa\tau} d^3r}; \int_0^\infty e^{-(x/a)^2} dx = a\sqrt{(\pi)}/2, \\
&\int_0^\infty x^2 e^{-(x/a)^2} dx = a^3\sqrt{(\pi)}/2^3 \\
&= 3\kappa\tau + \frac{\int_{r=0}^{\infty} \int_{\theta=0}^{\pi/2} \int_{\phi=0}^{2\pi} mgr\cos(\theta) \cdot e^{-mgr\cos(\theta)/\kappa\tau} r^2 \sin(\theta) dr d\theta d\phi}{\int_{r=0}^{\infty} \int_{\theta=0}^{\pi/2} \int_{\phi=0}^{2\pi} e^{-mgr\cos(\theta)/\kappa\tau} r^2 \sin(\theta) dr d\theta d\phi} \\
&= 3\kappa\tau + \frac{\int_{r=0}^{\infty} \int_{\theta=0}^{\pi/2} mgr\cos(\theta) \cdot e^{-mgr\cos(\theta)/\kappa\tau} r^2 \sin(\theta) dr d\theta}{\int_{r=0}^{\infty} \int_{\theta=0}^{\pi/2} e^{-mgr\cos(\theta)/\kappa\tau} r^2 \sin(\theta) dr d\theta} \\
&= 3\kappa\tau + \kappa\tau \frac{\int_{\rho=0}^{\infty} \int_{\lambda=0}^{1} \rho^3 \lambda \cdot e^{-\rho\lambda} d\rho d\lambda}{\int_{\rho=0}^{\infty} \int_{\lambda=0}^{1} \rho^2 \cdot e^{-\rho\lambda} d\rho d\lambda}; \rho = mgr/\kappa\tau, \lambda = \cos(\theta) \\
&= 3\kappa\tau + \kappa\tau \lim_{b\to 0} \frac{\int_{\lambda=b}^{1} \lambda(\frac{3!}{\lambda^4}) d\lambda}{\int_{\lambda=b}^{1} (\frac{2!}{\lambda^3}) d\lambda}; \int_0^\infty x^n e^{-ax} dx = n!/a^{n+1} \\
\langle \varepsilon_d \rangle &= 6\kappa\tau
\end{aligned}
\tag{9}
$$

## IV. DERIVATIONS OF ANGLES AND HEIGHT, EQ. (10)-(12)

Fig. S2 shows the Fig. 3(c) with more detailed labels. To get the integration window for $\acute{\phi}$, the maximum $\acute{\phi}_{max}$ is $\widehat{BCD}$ in Fig. S2. $\overline{BD} = \gamma_1 l/2$ and $\overline{CD} = \gamma_0 l/2$. Hence, $\widehat{BCD} = \tan^{-1}(\overline{BD}/\overline{CD}) = \tan^{-1}(\gamma_1/\gamma_0)$, i.e. eq. (10).

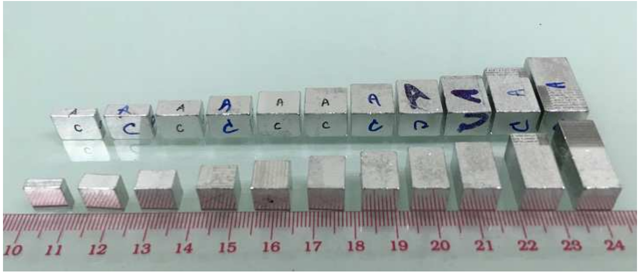


FIG. 3: Tetragonal and orthorhombic aluminium dice in various sizes.

To get the integration window for $\acute{\theta}$, the maximum $\acute{\theta}_{max}(\acute{\phi})$ as a function of $\acute{\phi}$ is $\widehat{CAG}$ in Fig. S2. $\overline{AC} = \gamma_2 l/2$ and $\overline{CG} = \gamma_0 l/2\cos(\acute{\phi})$. Hence, $\widehat{CAG} = \tan^{-1}(\overline{CG}/\overline{AC}) = \tan^{-1}(\gamma_0/\gamma_2\cos(\acute{\phi})$, i.e. eq. (11).

In Fig. S2, the height $h$ in eq. (12) can be written as:

$$h = \overline{AB}\cos(\alpha). \tag{10}$$

Using the dot product,

$$\cos(\alpha) = \overrightarrow{AB}\cdot\overrightarrow{AE}/\overline{AB}\cdot\overline{AE}. \tag{11}$$

By using this result,

$$h = \overline{AB}\cos(\alpha) = \overrightarrow{AB}\cdot\overrightarrow{AE}/\overline{AE}. \tag{12}$$

By using the die reference frame and setting point A to the origin (0, 0, 0), we can then define $\overrightarrow{AB} = \frac{l}{2}(\gamma_0, \gamma_1, \gamma_2)$ and $\overrightarrow{AE} = \frac{l}{2}(\gamma_2\tan(\acute{\theta})\cos(\acute{\phi}), \gamma_2\tan(\acute{\theta})\sin(\acute{\phi}), \gamma_2)$. $\overline{AE} = |\overrightarrow{AE}| = \gamma_2 l/2\cos(\acute{\phi})$.

Finally,

$$h = \overrightarrow{AB}\cdot\overrightarrow{AE}/\overline{AE} = \frac{l}{2}(\gamma_0\sin\acute{\theta}\cos\acute{\phi} + \gamma_1\sin\acute{\theta}\sin\acute{\phi} + \gamma_2\cos\acute{\theta}). \tag{13}$$

[1] Derivation of Boltzmann distribution is from the lecture note of Prof. Angel C de Dios; Also, H. A. Bent, "The Second Law," Oxford University Press, New York, 1965.
[2] J. Nagler and P. Richter, Phys. Rev. E. 78, 036207 (2008).
